# Supplementary material for: WANDR: Intention-guided Human Motion Generation
Source: arXiv:2404.15383 source file (2024-04-23)
Supplement: Supplementary file 1 [file 7_appendix.tex]

% \thesection instead of A would make it A.1, B.1...
\setcounter{figure}{0} 

\setcounter{table}{0} 

\appendix
