# Supplementary material for: WANDR: Intention-guided Human Motion Generation
Source: arXiv:2404.15383 source file (2024-04-23)
Supplement: Supplementary file 2 [file inbetween.tex]

\begin{figure*}[!h]
    \centering
    \includegraphics[width= 1.\textwidth, trim=0cm 0cm 0cm 0cm]{figures/traj_following.png}
    \caption{Demonstration of motion in-betweening during goal reaching, highlighting \methodname's capability to generate motions that conform to intermediate body poses while progressing towards a goal.}
    \label{fig:motion_inbetweening}
    % \vspace{-3mm}
\end{figure*}
