# Supplementary material for: WANDR: Intention-guided Human Motion Generation
Source: arXiv:2404.15383 source file (2024-04-23)
Supplement: Supplementary file 3 [file moving_goal.tex]

\begin{figure*}[!h]
    \centering
    \includegraphics[width= .9\textwidth, trim=0cm 0cm 0cm 0cm]{figures/moving_goal_dummy.png}
    \caption{moving goal reaching}
    \label{fig:moving_goal}
    % \vspace{-3mm}
\end{figure*}
