# Supplementary material for: WANDR: Intention-guided Human Motion Generation
Source: arXiv:2404.15383 source file (2024-04-23)
Supplement: Supplementary file 4 [file optimization_table.tex]

\begin{table}[tb]
\centering
% \small
% \resizebox{1.\linewidth}{!}{
\begin{tabular}{l|ccc}
\Xhline{2\arrayrulewidth}
\textbf{} & \textbf{SR $\uparrow$} & \textbf{FS $\downarrow$} & \textbf{DTG (cm) $\downarrow$} \\
\hline
\methodname        & KK\% & KK\% & KK \\
\methodname+opt.        & KK\% & KK\% & KK \\
\methodname+post opt.        & KK\% & KK\% & KK \\
\Xhline{2\arrayrulewidth}
\end{tabular}
% }
\caption{}
\vspace{-3mm}
\label{tab:optimization}
\end{table}
